# Supplementary material for: QUILL: Query Intent with Large Language Models using Retrieval Augmentation and Multi-stage Distillation
Source: arXiv:2210.15718 source file (2022-10-27)
Supplement: Supplementary file 1 [file 9_appendix.tex]

\section{Appendix 1}
\label{sec:appendix1}

We used the ORCAS-I Dataset's golden set as our test set.

The Retrieval Augmentation of these queries - addition of URLs and Titles -- were done by joining ORCAS and MS-MARCO datasets.

\section{Appendix 2}
\label{sec:appendix2}

Experiment Setup.
